# Supplementary material for: Selective Experience Replay for Lifelong Learning
Source: arXiv:1802.10269 source file (2018-02-28)
Supplement: Supplementary file 1 [file appendix.tex]

\appendix
\section{Appendix}\label{sec:appendix}
% MOVE DETAILS ABOUT SIMULATION ENVIRONMENT HERE
%scenarios and what they have in common, density,
\subsection{Simulation environment: SUMO} \label{sec:simulation}
% SIMULATION
The Sumo simulator \cite{sumo} is an open source traffic simulation package. This package allows users to model road networks, road signs, traffic lights, a variety of vehicles (including public transportation), and pedestrians. Importantly for the purpose of testing and evaluation of autonomous vehicle systems, Sumo provides tools that facilitate online interaction and vehicle control. For any traffic task, users can have control over a vehicle's position, velocity, acceleration, steering direction and can simulate motion using basic kinematics models. Traffic tasks like multi-lane intersections can be setup by defining the road network (lanes and intersections) along with specifications that control traffic conditions. To simulate traffic, users have control over the types of vehicles, road paths, vehicle density, and departure times. Traffic cars follow the intelligent driver model to control their motion. In Sumo, randomness is simulated by varying the speed distribution of the vehicles and by using parameters that control driver imperfection (based on the Krauss stochastic driving model \cite{krauss1998sumo}). The simulator runs based on a predefined time interval which controls the length of every step. 

The Sumo traffic simulator is configured so that each lane has a 45 miles per hour (20 m/s) max speed. The car begins from a stopped position. Each time step is equal to 0.2 seconds. The max number of steps per trial is capped 100 steps which is equivalent to 20 seconds. The traffic density is set by the probability that a vehicle will be emitted randomly per second. We use depart probability of 0.2 for \emph{each lane} for all tasks.

\subsection{Simulation environment: Grid World} \label{sec:gridworld}
The agent starts in the top left of a four room world sized $11 \times 11$. The agent's objective is to navigate to a goal in one of the other rooms. 
Figure \ref{fig:gridworld} Shows an example state in grid world. Each room corresponds to different task. The agent's action space consists of moving $\{up, down, left, right\}$. The agent is allowed up to $100$ steps per trial, and the agent trains for $10,000$ iterations for each task for a total of $30,000$ iterations. 

\begin{figure}[t]
\centering
\hspace{-10pt}
  \includegraphics[trim={0 0 0 10mm}, clip, width=0.5\textwidth]{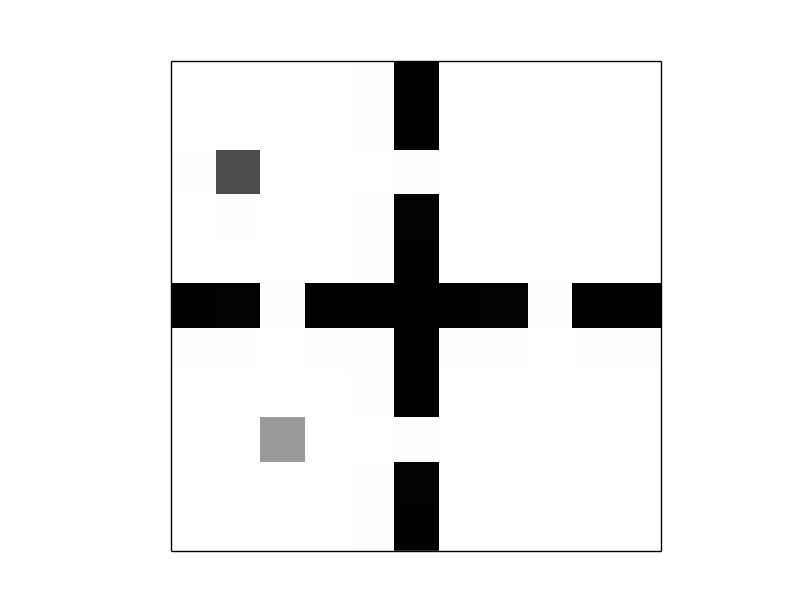}
  \caption{Grid world domain. Black indicates a wall, dark gray is the agent, and light gray is the goal.}
  \label{fig:gridworld}
  \vspace{-10pt}
\end{figure}

\subsection{Lifelong MNIST} \label{sec:mnist}

The popular MNIST dataset \cite{lecun1998gradient} has several extensions to lifelong learning problems 
\cite{alsharif2014lifelong,gaunt2017differentiable}. We turn the MNIST dataset into a lifelong learning problem by exposing the networks to only two digits at a time. We break the dataset into pairs by having task $i$ consist of the $i$ and $i+5$ digit, for example task $1$ will involve digits $1$ and $6$. This requires that the network remember how to classify previous digits in order to perform well on the entire dataset. Naively training on data as it arrives will generally destroy the representations built for the first task in order to learn the second. Each task is trained for $1000$ iterations. When mapping the selection strategies from a reinforcement problem to a classification problem reward would typically be associated with a correct classification. Since the network error is already being used by the surprise selection, we omit reward from the experiment as it would be redundant.

\subsection{Experimental Setup} \label{sec:setup}
%\input{driving}

%\FloatBarrier
   
% Network
The state space of the DQN is represented as a $18 \times 26$ grid in global coordinates from the intersection domain ($11 \times 11$ for grid world and $28 \times 28$ for MNIST). The DQN network uses a convolutional neural network with two convolution layers, and one fully connected layer. The first convolutional layer has $32$ $6 \times 6$ filters with stride two ($5 \times 5$ for MNIST), the second convolution layer has $64$ $3 \times 3$ filters with stride two ($5 \times 5$ for MNIST). The fully connected layer has 100 nodes. All layers use leaky ReLU activation functions \cite{maas2013rectifier}. The final linear output layer has outputs corresponding the domain specific action space. The network is optimized using the RMSProp algorithm \cite{tieleman2012lecture} (standard gradient descent for MNIST). 

% EXPERIENCE REPLAY
Our experience replay buffers have an allotment of $1,000$ experiences. The FIFO only trials have a single replay buffer with $1,000$ experiences. Networks using a selective replay buffer store $900$ experiences in the selective buffer and $100$ in the smaller FIFO buffer. At each learning iteration we samples a total batch size of 60 which is split as 30 experiences from each buffer when using selective replay. This means minibatches are even mix of data from both buffers.

Since the experience replay buffer imposes off-policy learning, we are able to calculate the return for each state-action pair in the trajectory prior to adding each step into the replay buffer. This allows us to train on the n-step return \cite{peng1996incremental}.% and forgo the addition of using target networks \cite{mnih2015human}.

Because surprise changes over the course of training, one can imagine implementing the surprise method to either hold on to the examples that were initially surprising, or to update samples with their new TD values as they are trained on. In the later case, the TD errors would shrink as the network learns the hard examples and they would eventually be removed from the buffer. In practice this is what we see, updating the TD errors eventually removes samples from older tasks until the buffer only has samples from the current task. This causes the network to forget earlier tasks, and in every domain we tried, we got better performance by holding on to the initial surprising examples. For this reason we show results from the method that holds on to initially surprising examples. 

The number of neighbors in coverage maximization is dependent on the samples currently in the buffer. As the buffer changes the number of a neighbors a sample has may also change. To accommodate the change in buffer distribution, an experience's score is updated when it is sampled for training.

For calculating the distances between experiences in the coverage maximization approach we concatenate all components of the experience (state, action, next state and reward) and use the extended Jaccard metric for the intersection domain because the state representation is sparse (cosine similar worked equally well). For the states in grid world we use the L1 distance between the different agents and the different goals. For MNIST we tried L2, although it did not work very well and we suspect this is the cause of the poor performance of coverage approach on MNIST, we also experimented with cosine and Jaccard, but these did not work any better.  
% We looked at computing the distances between the separate parts (i.e. state vs state, action vs action) to balance the contributions from each but weren't certain the contributions should be balanced (is the difference between action as important as the difference between state?) and empirically it didn't make a noticeable difference. We did observe ( looking at t-SNE projections) that incorporating action and reward did produce different grouping compared to using the distance between state only.

The epsilon governing random exploration was $0.05$.  
For the reward we used $+1$ for successfully navigating the intersection, $-1$ for a collision, and $-0.01$ step cost. 
Testing is run as separate procedure that does not have an impact on the replay buffer or the learning process of the network.

\section{Additional Experiments}

\subsection{Time Dependence of TD Error}
\begin{figure}[h!]
    \centering
    \hspace{-20pt}
    	\includegraphics[width=0.4\textwidth]{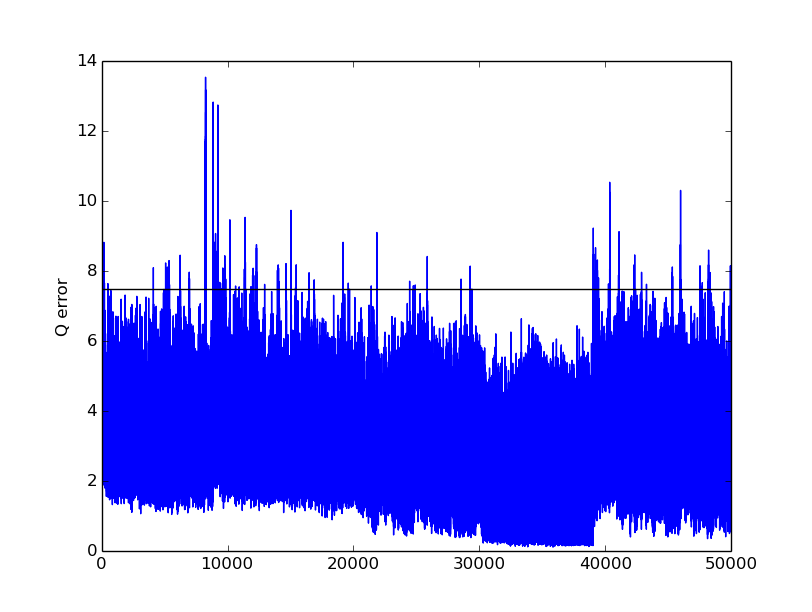}
        \caption{Max TD error during training. The samples above the black line are the samples in episodic memory at the end of training. Despite the fact that average TD error decreases during training, there are large TD throughout the learning process.}\label{fig:TDtrain} 
\end{figure}
Temporal Difference errors are dependent on the current state of the learning system and therefore have an implicit dependence on time. Since generally the error decreases during training we might assume that the magnitude of TD errors also decreases over time. We plot the max TD error during a typical training run in Figure \ref{fig:TDtrain}. We observe that even though the average error decreases over time, large TD errors exist throughout the learning process. The black line indicates the top 1000 errors.

\subsection{Empirically Investigating Coverage}

To verify that our maximum coverage selection process is in fact covering the state space, we run our selection process and then project the high dimensional experiences into two dimensions. This process is shown in Figure \ref{fig:tsne}. We see that the projected state space is projected into a sphere with simpler tasks with fewer lanes are projected in the center, and more challenging tasks with more lanes on the outside. As a result of the dimensionality reduction, we do not expect the selected points (shown in black) to be perfectly uniform, however we do observe the selected points cover most regions of the space. 

\begin{figure}[h!]
    \centering
    	\includegraphics[width=0.4\textwidth]{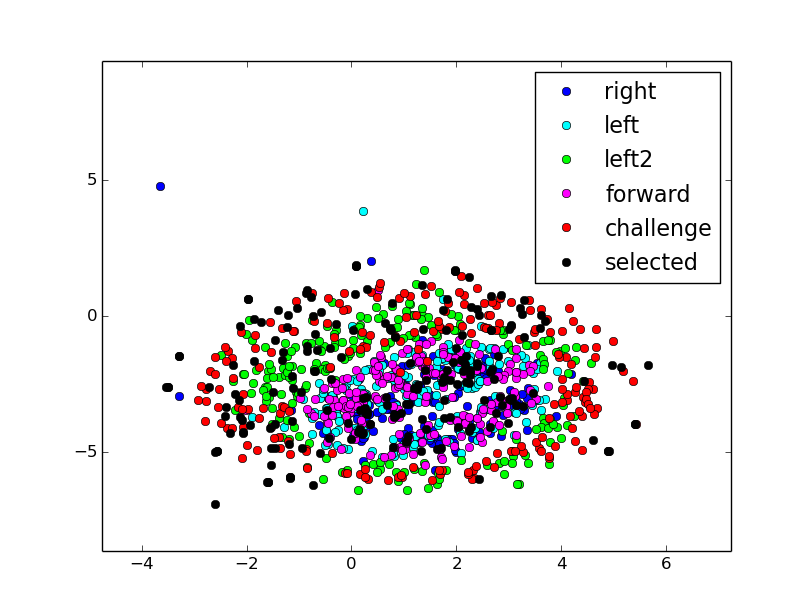}
  \caption{}
  \label{fig:tsne}  
        \caption{Projection of the state space using t-SNE \cite{maaten2008visualizing}. Points selected by our algorithm are shown in black. We see that our method gives good coverage across the state space.}\label{fig:tsne} 
\end{figure}

\subsection{Selective Replay Only}
We ran an experiment to evaluate the performance when training with only long term episodic memory, and not the short term FIFO buffer. Results are shown in Figure \ref{fig:only}. Training is stable and resistant to forgetting, however the performance is not as good as the performance of training with both storage mechanisms.

\begin{figure}[]
\centering
\hspace{-10pt}
  \includegraphics[trim={0 0 0 10mm}, clip, width=0.4\textwidth]{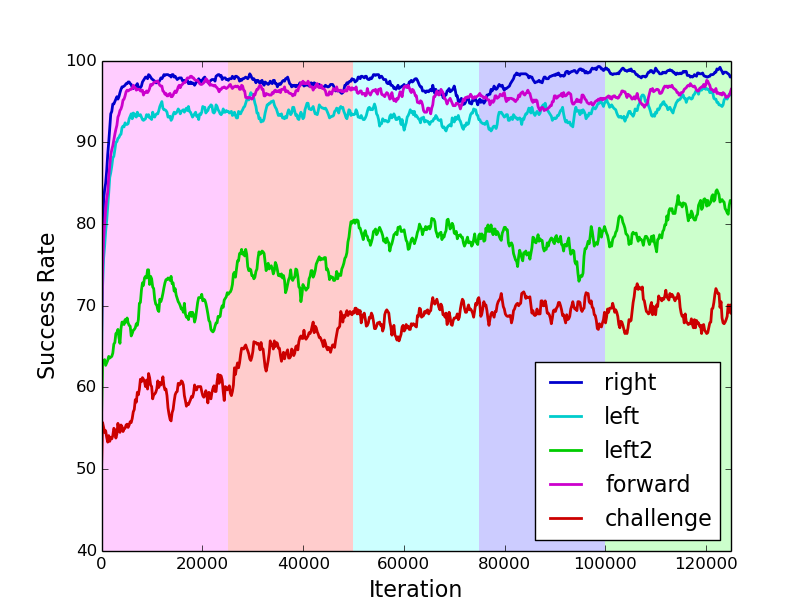}
  \caption{Performance using only a selective buffer. The performance impaired since the network is exposed to fewer examples. This is particularly noticeable in the more challenging cases.}
  \label{fig:only}
  \vspace{-10pt}
\end{figure}

\subsection{Distributions of Samples Stored in Buffer}

We looked at how many samples from each task were in the buffer at the end of training under the different approaches. Results are shown in Table \ref{table:experience_distribution}. Mistakes made by the network early in training were often smaller errors and have longer to get pushed out of the buffer, as a result the first task has few samples. The harder tasks (Left2 and Challenge) also appear to correlate with larger errors. Reward has balanced examples from each task, since each task has a fixed reward, although since long trials that result in a collision will have more negative reward than short failures, we see that Left2 and Challenge have slightly more samples. Coverage Maximization has a large variance on the number of samples for Right, Left2, and Forward. This is because they occupy a similar region in space, see Figure \ref{fig:tsne}. As a result, the buffer may have many samples of Right, and hold on to fewer for Left and Forward. However which task it held more samples for varied across trials, resulting in the large variance. Distribution Matching is balanced with more samples for Left2 and Challenge. This slight imbalance is due to the fact that the harder tasks tended to have longer trials, therefore producing more samples.

% GRID
% [ 21506.66666667  39956.          28537.33333333] [ 6925.55534075  2476.07693742  4451.69096462]
% [ 34499.          33949.33333333  21551.66666667] [  906.72175078  1026.666829    1931.72499193]
% [ 20278.          19211.66666667  50510.33333333] [ 1793.14704733  1360.68883699  3153.39422069]
% [ 27694.33333333  24648.66666667  37657.        ] [ 451.19446411  591.2062058   159.98229069]

% SUMO
% [   3.66666667   70.33333333  344.66666667   97.          384.33333333] [  0.8819171   19.67513942  64.11534744  23.43786111  33.57743952]
% [ 116.5  155.5  210.   153.5  264.5] [  4.5   5.5  16.   35.5   9.5]
% [ 221.33333333  163.33333333  108.66666667  106.33333333  300.33333333] [ 110.33333333   79.67085066  107.17016583  103.84336495   21.67435761]
% [ 117.          156.33333333  229.33333333  150.          247.33333333] [ 10.21436896  16.37409879  12.71918935  10.59874206  25.89937794]

\begin{table}[h!]
\caption{Distribution of Stored Experiences}
    \begin{tabular}{  l | l | l | l | l | l }
    Method & Right & Left & Left2 & Forward & Challenge \\ \hline
    Surprise & $4 \pm 1$  &  $70 \pm 20$  &  $345 \pm 60$  &  $97 \pm 20$  &  $384 \pm 30$\\
    Reward & $117 \pm 5$  &  $156 \pm 6$  &  $210 \pm 16$  &  $154 \pm 36$  &  $265 \pm 10$\\
    Coverage & $221 \pm 110$  &  $163 \pm 80$  &  $109 \pm 107$  &  $106 \pm 104$  &  $300 \pm 22$\\
    Matching & $117 \pm 10$  &  $156 \pm 16$  &  $229 \pm 13$  &  $150 \pm 11$  &  $247 \pm 26$\\
    \end{tabular}
    \label{table:experience_distribution}
\end{table}
